# Supplementary material for: Accurate and Scalable Stochastic Gaussian Process Regression via Learnable Coreset-based Variational Inference
Source: arXiv:2311.01409 source file (2025-03-04)
Supplement: Supplementary file 1 [file cvtgp_derivation_f_old.tex]

% !TEX root = ../main.tex



We derive below,
under the assumption of standard Gaussian observation noise\footnote{The derivations are equivalent for non-zero mean and/or correlated noise functions.},
\ie $\yb = \fb + \epsilon\;, \epsilon \sim \N{\epsilon\mid \zerob, \sigma^2 \Ib}$,
the coreset-based tempered posterior over $\gp$ coreset function values $q(\fbC)$.

% Function-space posterior coreset
\subsubsection{The coreset-based tempered-posterior}
\label{assec:cvtgp_qf_analytical}

To be able to accurately approximate the full $\gp$ posterior with a coreset $\{\XbC, \ybC \}$,
we propose to weight with $\beta_c \geq 0$ the likelihood of each coreset datapoint when computing their corresponding coreset $\gp$ value $\fbC$, \ie 

\begin{align}
	\cq{\fbC}{\XbC, \ybC, \betabC} &= \frac {\cq{\ybC}{\fbC, \betabC} \cp{\fbC}{\XbC}}{\cq{\ybC}{\XbC, \betabC} } 
		= \frac {\left(\prod_{m=1}^M \cp{y_{m}}{f_{m}}^{\beta_{m}} \right) \cp{\fbC}{\XbC}}{\cq{\ybC }{\XbC, \betabC} } \; .
\end{align}

In practice, we ensure positive $\beta_m$ using the $\mathrm{softplus}(.)$ function. We start by deriving a closed form expression for the $\betabC$-weighted likelihood function $q(\ybC | \fbC, \betabC)$,
by considering each coreset pair $\{x_{m},y_{m}\}$, for $m = 1, \cdots, M,$ independently,

\begin{align}
	\cq{y_m}{f_m, \beta_m} &= \cp{y_{m}}{f_{m}}^{\beta_{m}} = \N{y_{m} \mid f_{m}, \sigma^2}^{\beta_{m}} \\
	&= \left(\frac{1}{\sqrt{2 \pi \sigma^2}} e^{- \frac{1}{2} (y_{m} - f_{m}) \sigma^{-2} (y_{m} - f_{m})}\right)^{\beta_{m}} \\
	&= \left(\frac{1}{\sqrt{2 \pi \sigma^2}}\right)^{\beta_{m}} e^{- \frac{1}{2} (y_{m} - f_{m}) (\beta_{m}^{-1}\sigma^2)^{-1} (y_{m} - f_{m})} \\
	&= \left(\frac{1}{\sqrt{2 \pi \sigma^2}}\right)^{\beta_{m}}
	\left(\frac{\sqrt{2 \pi \beta_{m}^{-1}\sigma^2}}{\sqrt{2 \pi \beta_{m}^{-1}\sigma^2}}\right) \exp\left\{- \frac{1}{2} (y_{m} - f_{m}) (\beta_{m}^{-1}\sigma^2)^{-1} (y_{m} - f_{m})\right\} \\
        &= \frac{\sqrt{2 \pi \beta_{m}^{-1}\sigma^2}}{\left(\sqrt{2 \pi \sigma^2}\right)^{\beta_{m}}}
	\left(\frac{1}{\sqrt{2 \pi \beta_{m}^{-1}\sigma^2}}\right) \exp\left\{- \frac{1}{2} (y_{m} - f_{m}) (\beta_{m}^{-1}\sigma^2)^{-1} (y_{m} - f_{m})\right\} \\
        &= \frac{\sqrt{2 \pi \beta_{m}^{-1}\sigma^2}}{\left(\sqrt{2 \pi \sigma^2}\right)^{\beta_{m}}} \cdot \N{y_m|f_m, \beta_{m}^{-1}\sigma^2} \\
        &= Q_c \cdot \N{y_m|f_m, \beta_{m}^{-1}\sigma^2} \;, \\
        & \text{ with } Q_c = \frac{\sqrt{2 \pi \beta_{m}^{-1}\sigma^2}}{\left(\sqrt{2 \pi \sigma^2}\right)^{\beta_{m}}} \;.
\end{align}

We write the joint over the full coreset pseudo-observations as a product over each likelihood term
\begin{align}
	&q(\ybC | \fbC, \betabC) = \prod_{m=1}^M p(y_{m} | f_{m})^{\beta_{m}} \\
	& \qquad = \prod_{m=1}^M\left(\frac{1}{\sqrt{2 \pi \sigma^2}}\right)^{\beta_{m}}
	\left(\frac{\sqrt{2 \pi \beta_{m}^{-1}\sigma^2}}{\sqrt{2 \pi \beta_{m}^{-1}\sigma^2}}\right) \exp\left\{- \frac{1}{2} (y_{m} - f_{m}) (\beta_{m}^{-1}\sigma^2)^{-1} (y_{m} - f_{m})\right\} \\
        & \qquad = \prod_{m=1}^M Q_m \cdot \N{y_m|f_m, \beta_{m}^{-1}\sigma^2} \\
        & \qquad = Q_M \cdot \N{\ybC \mid \fbC, \Sigma_{\betabC}} \;, \text{ with }
        \begin{cases}
            Q_M = \prod_{m=1}^M\frac{\sqrt{2 \pi \beta_{m}^{-1}\sigma^2}}{\left(\sqrt{2 \pi \sigma^2}\right)^{\beta_{m}}}  \\
            \Sigma_{\betabC} = \sigma^2 \cdot \diag{\betabC^{-1}} 
        \end{cases} \;.
        \label{eq:coreset_likelihood}
\end{align}

We derive the marginalized pseudo-observation coreset distribution
\begin{align}
	q(\ybC|\XbC, \betabC) &= \int_{\fbC} q(\ybC, \fbC | \XbC, \betabC) \diff{\fbC} = \int_{\fbC} q(\ybC | \fbC, \betabC) p(\fbC|\XbC) \diff{\fbC} \\
        & = \int_{\fbC} Q_M \cdot \N{\ybC \mid \fbC, \Sigma_{\betabC}} \cdot \N{\fbC \mid \zerob, \Kb_{\XbC,\XbC}}  \diff{\fbC} \\
        & = Q_M \int_{\fbC} \N{\ybC \mid \fbC, \Sigma_{\betabC}} \cdot \N{\fbC \mid \zerob, \Kb_{\XbC,\XbC}}  \diff{\fbC} \\
        & = Q_M \cdot \N{\ybC \mid \zerob, \Kb_{\XbC,\XbC} + \Sigma_{\betabC}} \;.
	\label{eq:coreset_marginal_likelihood}
\end{align}

We leverage the above distributions to derive the coreset-based, tempered $\gp$ posterior
\begin{align}
	& q(\fbC|\XbC, \ybC, \betabC) = \frac {q(\ybC | \fbC, \betabC) q(\fbC|\XbC)}{q(\ybC | \XbC, \betabC) } 	\\
	& \qquad = \frac{
		Q_M \cdot \N{\ybC \mid \fbC, \Sigma_{\betabC}} 
		 \N{\fbC \mid \zerob, \Kb_{\XbC,\XbC}}
	}{
		Q_M \cdot \N{\ybC \mid \zerob, \Kb_{\XbC,\XbC} + \Sigma_{\betabC}} 
	} \\
        & \qquad = \frac{
		\N{\ybC \mid \fbC, \Sigma_{\betabC}} 
		 \N{\fbC \mid \zerob, \Kb_{\XbC,\XbC}}
	}{
		\N{\ybC \mid \zerob, \Kb_{\XbC,\XbC} + \Sigma_{\betabC}} 
	} \\
        &\qquad = \N{\fbC \mid \mb_{\fbC|\ybC}, \Kb_{\fbC|\ybC}} \;, \text{ with} \begin{cases}
		\mb_{\fbC|\ybC} = \Kb_{\fbC|\ybC} \left(
		\Sigma_{\betabC}^{-1} \ybC 
		\right) \\
		\Kb_{\fbC|\ybC} = \left( 
		\Kb_{\XbC,\XbC}^{-1} + \Sigma_{\betabC}^{-1}
		\right)^{-1}
	\end{cases}  \hspace*{-2ex} .
	\label{eq:coreset_posterior_fc}
\end{align}

The sufficient statistics of the coreset-based tempered variational posterior above can be rewritten as
\begin{align}
    q(\fbC|\XbC, \ybC, \betabC) &= \N{\fbC \mid \mb_{\fbC|\ybC}, \Kb_{\fbC|\ybC}} \;, \\
    &\text{ with}
     \begin{cases}
		\mb_{\fbC|\ybC} = \Kb_{\XbC,\XbC} \left( \Kb_{\XbC,\XbC} + \Sigma_{\betabC} \right)^{-1} \ybC \\
		\Kb_{\fbC|\ybC} = \Kb_{\XbC,\XbC} - \Kb_{\XbC,\XbC} \left( \Kb_{\XbC,\XbC} + \Sigma_{\betabC} \right)^{-1} \Kb_{\XbC,\XbC}  \\
                \qquad \qquad \text{by \href{https://en.wikipedia.org/wiki/Woodbury_matrix_identity}{Woodbury matrix identity}}  \; .
	\end{cases} 
\end{align}

\paragraph{The coreset-based tempered-posterior over $\gp$ function values.}
We now compute the variational posterior over $\gp$ values for any given data point $\Xb$,
by marginalizing the $\gp$'s prior-conditional over the coreset-based posterior, \ie

\begin{align}
    q(\fb|\XbC, \ybC) &= \int_{\fbC} p(\fb|\fbC) q(\fbC | \XbC, \ybC, \betabC) \diff{\fbC} \;.
\end{align}

The above is analytically solvable due to all the distributions being Gaussian:
\begin{align}
	q(\fbC|\XbC, \ybC, \betabC) &= \N{\fbC \mid \mb_{\fbC|\ybC}, \Kb_{\fbC|\ybC}} \;, \\
        & \text{ with} \begin{cases}
		\mb_{\fbC|\ybC} = \Kb_{\fbC|\ybC} \left( \Sigma_{\betabC}^{-1} \ybC \right) \\
		\Kb_{\fbC|\ybC} = \Kb_{\XbC,\XbC} - \Kb_{\XbC,\XbC} \left(\Kb_{\XbC,\XbC} + \Sigma_{\betabC}\right)^{-1} \Kb_{\XbC,\XbC} 
	\end{cases} \hspace*{-2ex},
	\\
	p(\fb|\fbC) &= \N{\fb \mid \mb_{\fb|\fbC}, \Kb_{\fb|\fbC}} \;, \\
        & \text{ with} \begin{cases}
		\mb_{\fb|\fbC} = \Kb_{\Xb,\XbC}\Kb_{\XbC,\XbC}^{-1} \fbC \\
		\Kb_{\fb|\fbC} = \Kb_{\Xb,\Xb} - \Kb_{\Xb,\XbC}\Kb_{\XbC,\XbC}^{-1} \Kb_{\XbC,\Xb}
	\end{cases} \hspace*{-2ex},
	\\
	q(\fb|\XbC, \ybC, \betabC) &= \N{\fb \mid \mb_{\fb|\ybC}, \Kb_{\fb|\ybC}} \;, \\
        & \text{ with} \begin{cases}
		\mb_{\fb|\ybC} = \Kb_{\Xb,\XbC}\Kb_{\XbC,\XbC}^{-1} \mb_{\fbC|\ybC} \\
		\Kb_{\fb|\ybC} = \Kb_{\fb|\fbC} + \Kb_{\Xb,\XbC}\Kb_{\XbC,\XbC}^{-1} \Kb_{\fbC|\ybC} \Kb_{\XbC,\XbC}^{-1} \Kb_{\XbC,\Xb} 
	\end{cases} \hspace*{-2ex}.
    \label{eq:coreset_posterior_f}
\end{align}

We elaborate on the sufficient statistics of $q(\fb|\XbC, \ybC, \betabC)$.
First, we rewrite the expected value as
\begin{align}
	\mb_{\fb|\ybC} &= \Kb_{\Xb,\XbC}\Kb_{\XbC,\XbC}^{-1} \mb_{\fbC|\ybC} \\
	&= \Kb_{\Xb,\XbC}\Kb_{\XbC,\XbC}^{-1} \Kb_{\fbC|\ybC} \Sigma_{\betabC}^{-1} \ybC \\
	&= \Kb_{\Xb,\XbC}\Kb_{\XbC,\XbC}^{-1} \left( \Kb_{\XbC,\XbC}^{-1} + \Sigma_{\betabC}^{-1} \right)^{-1} \Sigma_{\betabC}^{-1} \ybC \\
		& \qquad \text{ by using equivalence in Equation~\eqref{eq:equiv_1}} \nonumber \\
	&= \Kb_{\Xb,\XbC}\left( \Kb_{\XbC,\XbC} + \Sigma_{\betabC} \right)^{-1} \ybC  \; ,
\end{align} 

where we have made use of the following equivalences,
\begin{align}
    % Equiv1
    & \Kb_{\XbC,\XbC}^{-1} \left( \Kb_{\XbC,\XbC}^{-1} + \Sigma_{\betabC}^{-1} \right)^{-1} \Sigma_{\betabC}^{-1} \nonumber \\
        & \qquad = \Kb_{\XbC,\XbC}^{-1} \left( \Sigma_{\betabC} \Kb_{\XbC,\XbC}^{-1} + I_C \right)^{-1} 
            = \left( \Sigma_{\betabC} + \Kb_{\XbC,\XbC} \right)^{-1}
        \label{eq:equiv_1} \;, \\
    % Equiv2
    & \Sigma_{\betabC}^{-1} \left( \Kb_{\XbC,\XbC}^{-1} + \Sigma_{\betabC}^{-1} \right)^{-1} \Kb_{\XbC,\XbC}^{-1} \nonumber \\
        & \qquad = \Sigma_{\betabC}^{-1} \left( I_C + \Kb_{\XbC,\XbC}\Sigma_{\betabC}^{-1}  \right)^{-1} 
	= \left( \Sigma_{\betabC} + \Kb_{\XbC,\XbC} \right)^{-1}
		\label{eq:equiv_2} \;.
\end{align}

Second, for the covariance matrix, we write
\begin{align}
	\Kb_{\fb|\ybC} &= \Kb_{\fb|\fbC} + \Kb_{\Xb,\XbC}\Kb_{\XbC,\XbC}^{-1} \Kb_{\fbC|\ybC} \Kb_{\XbC,\XbC}^{-1} \Kb_{\XbC,\Xb}\\
	&= \Kb_{\Xb,\Xb} - \Kb_{\Xb,\XbC}\Kb_{\XbC,\XbC}^{-1} \Kb_{\XbC,\Xb} \nonumber \\
	& \qquad + \Kb_{\Xb,\XbC}\Kb_{\XbC,\XbC}^{-1} \left( \Kb_{\XbC,\XbC}^{-1} + \Sigma_{\betabC}^{-1} \right)^{-1} \Kb_{\XbC,\XbC}^{-1} \Kb_{\XbC,\Xb}\\
	& \qquad \qquad \text{ by using the \href{https://en.wikipedia.org/wiki/Woodbury_matrix_identity}{Woodbury matrix identity} for } \left( \Kb_{\XbC,\XbC}^{-1} + \Sigma_{\betabC}^{-1} \right)^{-1} \nonumber \\
	&= \Kb_{\Xb,\Xb} - \Kb_{\Xb,\XbC}\Kb_{\XbC,\XbC}^{-1} \Kb_{\XbC,\Xb} \nonumber  \\
	& \qquad + 
            \resizebox{0.8\textwidth}{!}{$
                \Kb_{\Xb,\XbC}\Kb_{\XbC,\XbC}^{-1} \left( \Kb_{\XbC,\XbC} - \Kb_{\XbC,\XbC} \left(\Kb_{\XbC,\XbC} + \Sigma_{\betabC}\right)^{-1} \Kb_{\XbC,\XbC}  \right) \Kb_{\XbC,\XbC}^{-1} \Kb_{\XbC,\Xb}
                $} \\
	&= \Kb_{\Xb,\Xb} - \Kb_{\Xb,\XbC}\Kb_{\XbC,\XbC}^{-1} \Kb_{\XbC,\Xb} \nonumber  \\
	& \qquad + \Kb_{\Xb,\XbC}\left( \Ib_M - \left(\Kb_{\XbC,\XbC} + \Sigma_{\betabC}\right)^{-1} \Kb_{\XbC,\XbC}  \right) \Kb_{\XbC,\XbC}^{-1} \Kb_{\XbC,\Xb}\\	
	&= \Kb_{\Xb,\Xb} - \Kb_{\Xb,\XbC}\Kb_{\XbC,\XbC}^{-1} \Kb_{\XbC,\Xb} \nonumber \\
	& \qquad + \Kb_{\Xb,\XbC}\Kb_{\XbC,\XbC}^{-1} \Kb_{\XbC,\Xb} \nonumber \\
        & \qquad - \Kb_{\Xb,\XbC} \left(\Kb_{\XbC,\XbC} + \Sigma_{\betabC}\right)^{-1} \Kb_{\XbC,\XbC} \Kb_{\XbC,\XbC}^{-1} \Kb_{\XbC,\Xb}\\
	&= \Kb_{\Xb,\Xb} - \Kb_{\Xb,\XbC} \left(\Kb_{\XbC,\XbC} + \Sigma_{\betabC}\right)^{-1} \Kb_{\XbC,\Xb}  \; .
\end{align}

\subsubsection{The Function-space Variational Lower-bound with the Coreset Variational Posterior}
\label{assec:cvtgp_qf_lowerbound}

We follow the variational inference view of the log-marginal likelihood maximization, \ie

\begin{align}
	\Loss &= \Loss\left(\yb\right) = \log \p{\yb} = \Ex{\q{\fb}}{\log \cp{\yb}{\fb}}  
	+ \kl{\q{\fb}}{\cp{\fb}{\yb}}
	- \kl{\q{\fb}}{\p{\fb}}  \; ,
	\label{eq:loss_data_marginal_again}
\end{align}

where we denote with $q(\cdot)$ a generic family of distributions over the $\gp$ model $f$, evaluated at certain points of interest $\Xb$, $\fb=f(\Xb)$. Our variational family $q(\fb)$ decomposes over disjoint sets of the input space,
and respects the prior-conditionals of the $\gp$ model with respect to the coreset-based input points and function values.
Specifically, for $\fbC=f(\XbC)$ and, with a slight abuse of notation, $\fb=f(\Xb)$ for $\Xb = \Xb \setminus \XbC$,
\begin{align}
	\p{\fb, \fbC} = \cp{\fb}{\fbC} \p{\fbC} \; \leftrightarrow \;
	\q{\fb, \fbC} = \cp{\fb}{\fbC} \q{\fbC} \;.
\end{align}

Hence, we can rewrite the marginal above as
\begin{align}
	\Loss{} =\log \p{\yb } &= \Ex{\q{\fb, \fbC}}{\log \p{\yb}{\fb}}  
	+ \kl{\q{\fb, \fbC}}{\cp{\fb, \fbC}{\yb}}
	- \kl{\q{\fb, \fbC}}{\p{\fb, \fbC}} \\
	& = \Ex{\q{\fb}}{\log \p{\yb}{\fb} }  
	+ \kl{\q{\fb, \fbC}}{\p{\fb, \fbC}{\yb}}
	- \kl{\q{\fbC}}{\p{\fbC}}  \; ,
	\label{eq:loss_data_marginal_condprior}
\end{align}

due to the following simplifications enabled by the proposed variational family obeying the $\gp$'s prior-conditional
\begin{align}
    \kl{q(\fb, \fbC)}{p(\fb, \fbC)}&= \int_{(\fb, \fbC)} q(\fb, \fbC) \log \frac{q(\fb, \fbC)}{p(\fb, \fbC)} \diff{\fb}\diff{\fbC} \\
    &= \int_{(\fb, \fbC)} q(\fb, \fbC) \log \frac{p(\fb|\fbC) q(\fbC)}{p(\fb|\fbC) p(\fbC)} \diff{\fb}\diff{\fbC} \\
    &= \int_{(\fb, \fbC)} q(\fb, \fbC) \log \frac{q(\fbC)}{p(\fbC)} \diff{\fb}\diff{\fbC} \\
    &= \int_{(\fbC)} q(\fbC) \log \frac{q(\fbC)}{p(\fbC)}  \diff{\fbC} \\
    &= \kl{q(\fbC)}{p(\fbC)} \;,
\end{align}

and the expectation over the observed data log-likelihood only depending on the $\gp$ values $\fb$:
\begin{align}
    \Ex{q(\fb, \fbC)}{\log p(\yb| \fb) }  & = \int_{(\fb, \fbC)} q(\fb, \fbC) \log p(\yb| \fb) \diff{\fb}\diff{\fbC} \\
     & = \int_{(\fb, \fbC)} q(\fb, \fbC) \log p(\yb| \fb) \diff{\fb}\diff{\fbC} \\
     & = \int_{(\fb)} q(\fb) \log p(\yb| \fb) \dd{\fb} \\
     & = \Ex{q(\fb)}{\log p(\yb| \fb) }  \; .
\end{align}

A more thorough derivation for both the finite and infinite input dimensionality cases is detailed in Chapter 3 by~\citet{Matthews2017}.

We proceed to compute the loss of interest in Equation~\eqref{eq:loss_data_marginal_condprior}
by substituting the coreset-based tempered variational distributions in Equations~\eqref{eq:coreset_posterior_fc} and~\eqref{eq:coreset_posterior_f}. 

We start with the expectation of the data log-likelihood over the coreset-based posterior:
\begin{align}
	&\Ex{q(\fb|\XbC, \ybC, \betabC)}{\log p(\yb| \fb) } = \int_{\fb} q(\fb|\XbC, \ybC, \betabC) \log p(\yb| \fb ) \dd \fb \\
	& \qquad = \int_{\fb} q(\fb|\XbC, \ybC, \betabC) \log \N{\yb \mid \fb, \sigma^2 \Ib_N } \dd \fb \\
	& \qquad = \int_{\fb} q(\fb|\XbC, \ybC, \betabC)
	\left( 
	-\frac{N}{2}\log(2\pi) -\frac{1}{2} \log |\sigma^2 \Ib_N  | - \frac{1}{2}(\yb-\fb)^\top (\sigma^2\Ib_N)^{-1}(\yb-\fb)
	\right) \dd \fb \\
	& \qquad = -\frac{N}{2}\log(2\pi) 
	-\frac{1}{2} \log |\sigma^2 \Ib_N  |
	- \frac{1}{2\sigma^2} \int_{\fb} q(\fb|\XbC, \ybC,\betabC)
	\left(
	(\yb-\fb)^\top (\yb-\fb)
	\right) \dd \fb \\
	& \qquad = -\frac{N}{2}\log(2\pi) 
	-\frac{1}{2} \log |\sigma^2 \Ib_N  |
	- \frac{1}{2\sigma^2} \int_{\fb} q(\fb|\XbC, \ybC, \betabC)
	\left(
	\yb^\top\yb-2\yb^\top\fb+\fb^\top\fb
	\right) \dd \fb \\
	& \qquad = -\frac{N}{2}\log(2\pi) 
	-\frac{1}{2} \log |\sigma^2 \Ib_N  |
	- \frac{1}{2\sigma^2} \yb^\top\yb  \\
	& \qquad \qquad + \frac{2\yb^\top}{2\sigma^2} \int_{\fb} \fb q(\fb|\XbC, \ybC, \betabC) \dd \fb
		- \frac{1}{2\sigma^2} \int_{\fb} \left(
			\fb^\top\fb
		\right) q(\fb|\XbC, \ybC, \betabC) \dd \fb
	\\
	% Newline
	& \quad\text{ using the solution \href{https://statproofbook.github.io/P/mean-qf}{to the expectation of a quadratic from} } \\
	& \qquad = -\frac{N}{2}\log(2\pi) 
	-\frac{1}{2} \log |\sigma^2 \Ib_N  |
	- \frac{1}{2\sigma^2} \yb^\top\yb
	+ \frac{2\yb^\top}{2\sigma^2} \mb_{\fb|\ybC} \nonumber \\
        & \qquad \qquad - \frac{1}{2\sigma^2} \left( \mb_{\fb|\ybC}^\top \mb_{\fb|\ybC} + \tr{\Kb_{\fb|\ybC}}\right)\\
	% Newline
        & \qquad = -\frac{N}{2}\log(2\pi) 
	-\frac{1}{2} \log |\sigma^2 \Ib_N  |
	- \frac{1}{2\sigma^2} 
	\left( \yb^\top\yb
	- 2\yb^\top\mb_{\fb|\ybC}
	+ \mb_{\fb|\ybC}^\top \mb_{\fb|\ybC} \right) \nonumber \\
	& \qquad \qquad - \frac{1}{2 \sigma^2}\tr{\Kb_{\fb|\ybC}} \\
	& \qquad = \log \N{\yb \mid \mb_{\fb|\ybC}, \sigma^2 \Ib_N }
	- \frac{1}{2 \sigma^2}\tr{\Kb_{\fb|\ybC}}  \; .
	\label{eq:loss_coreset_posterior_gp_expectedloglik} 
\end{align}

We finally compute the KL term between the the coreset-based $\gp$ posterior and the $\gp$ prior over the coreset datapoints,
which are both Gaussian distributions of dimensionality $C$,
\begin{align}
	& \kl{q(\fbC|\XbC, \ybC, \betabC)}{p(\fbC)} = \kl{\N{\fbC \mid \mb_{\fbC|\ybC}, \Kb_{\fbC|\ybC}}}{\N{\fbC\mid \zerob, \Kb_{\XbC,\XbC}}} \\
	& \qquad = \frac {1}{2} \left(
		\tr{\Kb_{\XbC,\XbC}^{-1}\Kb_{\fbC|\ybC}} - C 
		+ \mb_{\fbC|\ybC}^\top \Kb_{\XbC,\XbC}^{-1}\mb_{\fbC|\ybC} 
		+ \log \left(\frac{|\Kb_{\XbC,\XbC}|}{|\Kb_{\fbC|\ybC}|}\right)
	\right) \;.
\end{align}

Let us elaborate separately on each term
\begin{align}
	\tr{\Kb_{\XbC,\XbC}^{-1}\Kb_{\fbC|\ybC}}
	& = \tr{\Kb_{\XbC,\XbC}^{-1}\left( \Kb_{\XbC,\XbC}^{-1} + \Sigma_{\betabC}^{-1} \right)^{-1}} \\
	% newline
	& = \tr{ \Kb_{\XbC,\XbC}^{-1} \Kb_{\XbC,\XbC} \left( \Ib_M - \left(\Kb_{\XbC,\XbC} + \Sigma_{\betabC}\right)^{-1} \Kb_{\XbC,\XbC} \right)} \\
	% newline
	& = \tr{\Ib_M - \left(\Kb_{\XbC,\XbC} + \Sigma_{\betabC}\right)^{-1} \Kb_{\XbC,\XbC}} \\
	% newline
	& = \tr{\Ib_M\}} - \tr{\left(\Kb_{\XbC,\XbC} + \Sigma_{\betabC}\right)^{-1} \Kb_{\XbC,\XbC}}  \\
	% newline
	& = C - \tr{\left(\Kb_{\XbC,\XbC} + \Sigma_{\betabC}\right)^{-1} \Kb_{\XbC,\XbC} }   \; .
	\label{eq:loss_coreset_posterior_gp_kl_trace}
\end{align}

\begin{align}
	&\mb_{\fbC|\ybC}^\top \Kb_{\XbC,\XbC}^{-1}\mb_{\fbC|\ybC} \\
        & \qquad = \left( \left( \Kb_{\XbC,\XbC}^{-1} + \Sigma_{\betabC}^{-1} \right)^{-1} \Sigma_{\betabC}^{-1} \ybC \right)^\top
	\Kb_{\XbC,\XbC}^{-1}
	\left( \left( \Kb_{\XbC,\XbC}^{-1} + \Sigma_{\betabC}^{-1} \right)^{-1} \Sigma_{\betabC}^{-1} \ybC \right) \\
	% newline
	& \qquad = \ybC^\top \Sigma_{\betabC}^{-1} \left( \Kb_{\XbC,\XbC}^{-1} + \Sigma_{\betabC}^{-1} \right)^{-1} 
	\Kb_{\XbC,\XbC}^{-1}
	\left( \Kb_{\XbC,\XbC}^{-1} + \Sigma_{\betabC}^{-1} \right)^{-1} \Sigma_{\betabC}^{-1} \ybC  \\
	% newline
	& \qquad = \ybC^\top \left( \Sigma_{\betabC}^{-1} \left( \Kb_{\XbC,\XbC}^{-1} + \Sigma_{\betabC}^{-1} \right)^{-1} \right)
	\left( \Kb_{\XbC,\XbC}^{-1} \left( \Kb_{\XbC,\XbC}^{-1} + \Sigma_{\betabC}^{-1} \right)^{-1} \Sigma_{\betabC}^{-1} \right) \ybC  \\
	% newline explation
	& \qquad \qquad \text{ by applying Equations~\eqref{eq:equiv_2} and~\eqref{eq:equiv_1} respectively} \nonumber \\
	% newline
	& \qquad = \ybC^\top 
		\left(\left( \Sigma_{\betabC} + \Kb_{\XbC,\XbC} \right)^{-1} \Kb_{\XbC,\XbC} \right)
		\left(\left( \Sigma_{\betabC} + \Kb_{\XbC,\XbC} \right)^{-1} \right)
		\ybC  \\
	& \qquad = \ybC^\top \left( \Sigma_{\betabC} + \Kb_{\XbC,\XbC} \right)^{-1} \Kb_{\XbC,\XbC} \left( \Sigma_{\betabC} + \Kb_{\XbC,\XbC} \right)^{-1} \ybC   \; .
	\label{eq:loss_coreset_posterior_gp_kl_quadratic}
\end{align}

\begin{align}
	\log \left(\frac{\left| \Kb_{\XbC,\XbC} \right|}{\left|\Kb_{\fbC|\ybC}\right|}\right)
	& = \log \left(\frac{\left|\Kb_{\XbC,\XbC}\right|}{\left| \left( \Kb_{\XbC,\XbC}^{-1} + \Sigma_{\betabC}^{-1} \right)^{-1} \right|}\right) \\
	% newline explation
	& \qquad \text{ by applying Equation~\eqref{eq:equiv_1}} \nonumber \\
	% newline
	& = \log \left(\frac{\left|\Kb_{\XbC,\XbC}\right|}{\left|\Kb_{\XbC,\XbC} \left( \Sigma_{\betabC} + \Kb_{\XbC,\XbC} \right)^{-1} \Sigma_{\betabC} \right|}\right) \\
	% newline
	& = \log \left(\frac{\left|\Kb_{\XbC,\XbC}\right|}{\left|\Kb_{\XbC,\XbC}\right| \left|\left( \Sigma_{\betabC} + \Kb_{\XbC,\XbC} \right)^{-1} \right| \left|\Sigma_{\betabC} \right|}\right) \\
	% newline
	& = + \log \left|\left( \Sigma_{\betabC} + \Kb_{\XbC,\XbC} \right)\right| - \log \left|\Sigma_{\betabC} \right|  \; .
	\label{eq:loss_coreset_posterior_gp_kl_logdet}
\end{align}

We put all terms together into a KL of the form

\begin{align}
	& \kl{q(\fbC|\XbC, \ybC, \betabC)}{p(\fbC)} \\
	& \qquad = \frac {1}{2} \left( \tr{ \Kb_{\XbC,\XbC}^{-1}\Kb_{\fbC|\ybC}} - C \right. \nonumber \\
	& \qquad \qquad + \mb_{\fbC|\ybC}^\top \Kb_{\XbC,\XbC}^{-1}\mb_{\fbC|\ybC} \nonumber \\
	& \qquad \qquad + \left. \log \left(\frac{|\Kb_{\XbC,\XbC}|}{|\Kb_{\fbC|\ybC}|}\right)  \right) \\
	% Newline
        & \qquad = \frac {1}{2} \left( C - \tr{ \left(\Kb_{\XbC,\XbC} + \Sigma_{\betabC}\right)^{-1} \Kb_{\XbC,\XbC}}  - C  \right. \nonumber \\
	& \qquad \qquad + \ybC^\top \left( \Sigma_{\betabC} + \Kb_{\XbC,\XbC} \right)^{-1} \Kb_{\XbC,\XbC} \left( \Sigma_{\betabC} + \Kb_{\XbC,\XbC} \right)^{-1} \ybC \nonumber  \\
	& \qquad \qquad + \left. \log \left|\left( \Sigma_{\betabC} + \Kb_{\XbC,\XbC} \right)\right| - \log \left|\Sigma_{\betabC} \right|  \right) \\
	% Newline
        & \qquad = \frac {1}{2} \left( - \tr{ \left(\Kb_{\XbC,\XbC} + \Sigma_{\betabC}\right)^{-1} \Kb_{\XbC,\XbC}} \right. \nonumber \\
	& \qquad \qquad + \ybC^\top \left( \Sigma_{\betabC} + \Kb_{\XbC,\XbC} \right)^{-1} \Kb_{\XbC,\XbC} \left( \Sigma_{\betabC} + \Kb_{\XbC,\XbC} \right)^{-1} \ybC \nonumber  \\
	& \qquad \qquad + \left. \log \left|\left( \Sigma_{\betabC} + \Kb_{\XbC,\XbC} \right)\right| - \log \left|\Sigma_{\betabC} \right| \right)  \; .
	\label{eq:loss_coreset_posterior_gp_kl}
\end{align}

We conclude with putting it all together as

\begin{align}
	\Loss_{CVGP(\fb)} & = \Ex{q(\fb)}{\log p(\yb| \fb) }  
	- \kl{q(\fbC)}{p(\fbC)}  \\
        % Newline
        & = \log \N{\yb \mid \mb_{\fb|\ybC}, \sigma^2 \Ib} - \frac{1}{2 \sigma^2}\tr{ \Kb_{\fb|\ybC}} \nonumber \\
        & \qquad - \frac {1}{2} \left( - \tr{ \left(\Kb_{\XbC,\XbC} + \Sigma_{\betabC}\right)^{-1} \Kb_{\XbC,\XbC} } \right. \nonumber \\
	& \qquad \qquad  + \ybC^\top \left( \Kb_{\XbC,\XbC} + \Sigma_{\betabC}\right)^{-1} \Kb_{\XbC,\XbC} \left( \Kb_{\XbC,\XbC} + \Sigma_{\betabC} \right)^{-1} \ybC \nonumber  \\
	& \qquad \qquad + \left. \log \left|\left( \Kb_{\XbC,\XbC} + \Sigma_{\betabC} \right)\right| - \log \left|\Sigma_{\betabC} \right| \right) \; .
        \label{eq:loss_cvtgp_analytical}
\end{align}

Importantly, the above loss is amenable to data-subsampling due to 
the properties of the trace and the diagonal covariance structure of the multivariate Gaussian $\N{\yb \mid \mb_{\fb|\ybC}, \sigma^2 \Ib}$,
\ie 

\begin{align}
	\Loss_{CVGP(\fb)} & = N\Ex{(\xb_i, y_i)\sim\mathcal{D}}{\log \N{y_i \mid m_{f_i|\ybC}, \sigma^2} - \frac{1}{2\sigma^{2}} k_{f_i,f_i|\ybC} } \nonumber \\
        & \qquad - \frac {1}{2} \left( - \tr{ \left(\Kb_{\XbC,\XbC} + \Sigma_{\betabC}\right)^{-1} \Kb_{\XbC,\XbC} } \right. \nonumber \\
	& \qquad \qquad  + \ybC^\top \left( \Kb_{\XbC,\XbC} + \Sigma_{\betabC}\right)^{-1} \Kb_{\XbC,\XbC} \left( \Kb_{\XbC,\XbC} + \Sigma_{\betabC} \right)^{-1} \ybC \nonumber  \\
	& \qquad \qquad + \left. \log \left|\left( \Kb_{\XbC,\XbC} + \Sigma_{\betabC} \right)\right| - \log \left|\Sigma_{\betabC} \right| \right)  \; ,
    \label{eq:loss_cvtgp_analytical_subsampling}
 \end{align}
 
where we have defined

\begin{align}
    m_{f_i|\ybC} &= \kb_{\xb_i, \XbC}\left( \Kb_{\XbC, \XbC} + \Sigma_{\betabC} \right)^{-1}\ybC \;, 
    \label{eq:data_likelihood_mean_xi} \\
    k_{f_i,f_i|\ybC}&= k_{\xb_i, \xb_i} - \kb_{\xb_i, \XbC}\left( \Kb_{\XbC, \XbC} + \Sigma_{\betabC} \right)^{-1} \kb_{\XbC, \xb_i} \; .
    \label{eq:data_likelihood_var_xi}
\end{align}

\subsubsection{The alternative function-space variational lower-bound with the Coreset-based Tempered-Posterior}
\label{assec:cvtgp_qf_lowerbound_2}

We revisit the loss of interest in Equation~\eqref{eq:loss_data_marginal_condprior} 
\begin{align}
	\Loss{} & = \Ex{q(\fb)}{\log p(\yb| \fb) }  
	+ \kl{q(\fb, \fbC)}{p(\fb, \fbC|\yb)}
	- \kl{q(\fbC)}{p(\fbC)} \\
        &\geq \Loss_{CVGP}{} = \Ex{q(\fb)}{\log p(\yb| \fb) } 
	- \kl{q(\fbC)}{p(\fbC)}  \; ,
\end{align}
and, as suggested by a NeurIPS2023 anonymous reviewer, directly replace the proposed coreset-based variational family
\begin{align}
	q(\fbC |\XbC, \ybC, \betabC ) &= \frac {q(\ybC | \fbC, \betabC) p(\fbC|\XbC)}{q(\ybC | \XbC, \betabC) } \;,
\end{align}
in the KL penalty term of CVGP's loss:
\begin{align}
	\Loss_{CVGP}{} &= \Ex{q(\fb|\XbC, \ybC, \betabC)}{\log p(\yb|\fb) } - \kl{q(\fbC|\XbC, \ybC, \betabC)}{p(\fbC|\XbC)} \\
        &= \Ex{q(\fb)|\XbC, \ybC, \betabC}{\log p(\yb| \fb) } - \Ex{q(\fbC|\XbC, \ybC, \betabC)}{\log \frac{q(\fbC|\XbC, \ybC, \betabC)}{p(\fbC|\XbC)}}\\
        &= \Ex{q(\fb|\XbC, \ybC, \betabC)}{\log p(\yb| \fb) } - \Ex{q(\fbC|\XbC, \ybC, \betabC)}{\log \frac{\frac {q(\ybC | \fbC, \betabC) p(\fbC|\XbC)}{q(\ybC | \XbC, \betabC) })}{p(\fbC|\XbC)}}\\
        &= \Ex{q(\fb|\XbC, \ybC, \betabC)}{\log p(\yb| \fb) } - \Ex{q(\fbC|\XbC, \ybC, \betabC)}{\log \frac{q(\ybC | \fbC, \betabC))}{q(\ybC | \XbC, \betabC)}}\\
        &= \Ex{q(\fb|\XbC, \ybC, \betabC)}{\log p(\yb| \fb) } - \Ex{q(\fbC|\XbC, \ybC, \betabC)}{\log q(\ybC | \fbC, \betabC))} + \Ex{q(\fbC|\XbC, \ybC, \betabC)}{\log q(\ybC | \XbC, \betabC)}\\
        &= \Ex{q(\fb|\XbC, \ybC, \betabC)}{\log p(\yb| \fb) } - \Ex{q(\fbC|\XbC, \ybC, \betabC)}{\log q(\ybC | \fbC, \betabC))} + \log q(\ybC | \XbC, \betabC) \;.
\end{align}

To elaborate on the above,
we note that the first term is provided by Equation~\eqref{eq:loss_coreset_posterior_gp_expectedloglik}
and that the second term can be derived similarly,
where to compute the expectation we use the coreset variational posterior $q(\fbC|\XbC, \ybC, \betabC)$ in Equation~\eqref{eq:coreset_posterior_fc}
and the coreset pseudo-likelihood follows $p(\ybC| \fbC, \betabC)=Q_M \cdot \N{\ybC \mid \fbC, \Sigma_{\betabC}}$ as in Equation~\eqref{eq:coreset_likelihood}:
\begin{align}
	&\Ex{q(\fbC|\XbC, \ybC, \betabC)}{\log p(\ybC| \fbC, \betabC) } = \int_{\fbC} q(\fbC|\XbC, \ybC, \betabC) \log p(\ybC| \fbC, \betabC) \dd \fbC \\
	& \qquad = \int_{\fbC} q(\fbC|\XbC, \ybC, \betabC) \log \left(Q_M \cdot \N{\ybC \mid \fbC, \Sigma_{\betabC} }\right) \dd \fbC \\
        & \qquad = \int_{\fbC} q(\fbC|\XbC, \ybC, \betabC) \left( \log Q_M + \log \N{\ybC \mid \fbC, \Sigma_{\betabC} } \right) \dd \fbC \\
        & \qquad = \log Q_M + \int_{\fbC} q(\fbC|\XbC, \ybC, \betabC) \log \N{\ybC \mid \fbC, \Sigma_{\betabC} } \dd \fbC \\
	& \qquad = \log Q_M +\int_{\fb} q(\fbC|\XbC, \ybC, \betabC)
	\left( 
	-\frac{C}{2}\log(2\pi) -\frac{1}{2} \log |\Sigma_{\betabC} | - \frac{1}{2}(\ybC-\fbC)^\top \Sigma_{\betabC}^{-1}(\ybC-\fbC)
	\right) \dd \fbC \\
	& \qquad = \log Q_M -\frac{C}{2}\log(2\pi) -\frac{1}{2} \log |\Sigma_{\betabC} |
	- \frac{1}{2} \int_{\fbC} q(\fbC|\XbC, \ybC,\betabC)
	\left(
	(\ybC-\fbC)^\top \Sigma_{\betabC}^{-1}(\ybC-\fbC)
	\right) \dd \fbC \\
        & \qquad = \log Q_M -\frac{C}{2}\log(2\pi) -\frac{1}{2} \log |\Sigma_{\betabC} |
	- \frac{1}{2} \Ex{q(\fbC|\XbC, \ybC,\betabC)}{
	(\ybC-\fbC)^\top \Sigma_{\betabC}^{-1}(\ybC-\fbC)
	}\\
        % Newline
	& \quad\text{ using the solution \href{https://statproofbook.github.io/P/mean-qf}{to the expectation of a quadratic from} with} \\
        & \qquad \begin{cases}
            \Ex{q(\fbC|\XbC, \ybC, \betabC)}{(\ybC-\fbC)} = (\ybC-\mb_{\fbC|\ybC}) \\
            \Cov_{q(\fbC|\XbC, \ybC, \betabC)}{(\ybC-\fbC)}=\Kb_{\fbC|\ybC}
        \end{cases} \\
	& \qquad = \log Q_M -\frac{C}{2}\log(2\pi) -\frac{1}{2} \log |\Sigma_{\betabC} |
	- \frac{1}{2} \left(
            (\ybC-\mb_{\fbC|\ybC})^\top \Sigma_{\betabC}^{-1}(\ybC-\mb_{\fbC|\ybC})
            + \tr{ \Sigma_{\betabC}^{-1} \Kb_{\fbC|\ybC}}
        \right) \\
        % Newline
        & \qquad = \log Q_M  \\
        & \qquad \qquad -\frac{C}{2}\log(2\pi) -\frac{1}{2} \log |\Sigma_{\betabC} |
	- \frac{1}{2} (\ybC-\mb_{\fbC|\ybC})^\top \Sigma_{\betabC}^{-1}(\ybC-\mb_{\fbC|\ybC}) \\
        & \qquad \qquad - \frac{1}{2} \tr{ \Sigma_{\betabC}^{-1} \Kb_{\fbC|\ybC}} \\
        % Newline
        & \qquad = \log Q_M  + \log \N{\ybC | \mb_{\fbC|\ybC}, \Sigma_{\betabC}} - \frac{1}{2} \tr{ \Sigma_{\betabC}^{-1} \Kb_{\fbC|\ybC}} \;.
\end{align}

By replacing the above expression in the lower-bound of interest,
along with the coreset marginalized likelihood in Equation~\eqref{eq:coreset_marginal_likelihood}, we conclude
\begin{align}
	\Loss_{CVGP}{} 
        &= \Ex{q(\fb|\XbC, \ybC, \betabC)}{\log p(\yb| \fb) } - \Ex{q(\fbC|\XbC, \ybC, \betabC)}{\log q(\ybC | \fbC, \betabC))} + \log q(\ybC | \XbC, \betabC) \\
        &= \log \N{\yb \mid \mb_{\fb|\ybC}, \sigma^2 \Ib} - \frac{1}{2 \sigma^2}\tr{\Kb_{\fb|\ybC}} \\
        & \qquad - \left( \log Q_M  + \log \N{\ybC | \mb_{\fbC|\ybC}, \Sigma_{\betabC}} - \frac{1}{2} \tr{ \Sigma_{\betabC}^{-1} \Kb_{\fbC|\ybC}} \right) \\
        & \qquad + \left( \log Q_M + \log N(\ybC | \zerob, \Kb_{\XbC,\XbC} + \Sigma_{\betabC}) \right) \\
        % Newline
        &= \log \N{\yb \mid \mb_{\fb|\ybC}, \sigma^2 \Ib} - \frac{1}{2 \sigma^2}\tr{\Kb_{\fb|\ybC}} \\
        & \qquad - \log \N{\ybC | \mb_{\fbC|\ybC}, \Sigma_{\betabC}} + \frac{1}{2} \tr{ \Sigma_{\betabC}^{-1} \Kb_{\fbC|\ybC}}  \\
        & \qquad + \log N(\ybC | \zerob, \Kb_{\XbC,\XbC} + \Sigma_{\betabC}) \\
        % Newline
        &= \log \N{\yb \mid \mb_{\fb|\ybC}, \sigma^2 \Ib} - \frac{1}{2 \sigma^2}\tr{\Kb_{\fb|\ybC} } \\
        & \qquad + \frac{1}{2} \tr{
            \Sigma_{\betabC}^{-1} \left( \Kb_{\XbC,\XbC}^{-1} + \Sigma_{\betabC}^{-1} \right)^{-1}}  \\
        & \qquad - \left( -\frac{C}{2} \log (2\pi) - \frac{1}{2} \log\left|\Sigma_{\betabC}\right| -\frac{1}{2} (\ybC-\mb_{\fbC|\ybC})^\top \Sigma_{\betabC}^{-1}(\ybC-\mb_{\fbC|\ybC}) \right) \\
        & \qquad + \left( -\frac{C}{2} \log (2\pi) - \frac{1}{2} \log\left|\Kb_{\XbC,\XbC} + \Sigma_{\betabC} \right| -\frac{1}{2} \ybC^\top (\Kb_{\XbC,\XbC} + \Sigma_{\betabC})^{-1}\ybC\right) \\
        % Newline
        &= \log \N{\yb \mid \mb_{\fb|\ybC}, \sigma^2 \Ib} - \frac{1}{2 \sigma^2}\tr{\Kb_{\fb|\ybC}} \\
        & \qquad + \frac{1}{2} \tr{
            \left( \Kb_{\XbC,\XbC} + \Sigma_{\betabC} \right)^{-1} \Kb_{\XbC,\XbC}}  \\
        & \qquad + \frac{1}{2} \log\left|\Sigma_{\betabC}\right| - \frac{1}{2} \log\left|\Kb_{\XbC,\XbC} + \Sigma_{\betabC}\right| \\
        & \qquad + \frac{1}{2} \left[ (\ybC-\mb_{\fbC|\ybC})^\top \Sigma_{\betabC}^{-1}(\ybC-\mb_{\fbC|\ybC}) - \ybC^\top (\Kb_{\XbC,\XbC} + \Sigma_{\betabC})^{-1}\ybC \right ]
         \label{eq:data_quadratic_long}\\
        % Newline
        &= \log \N{\yb \mid \mb_{\fb|\ybC}, \sigma^2 \Ib} - \frac{1}{2 \sigma^2}\tr{\Kb_{\fb|\ybC}} \\
        & \qquad + \frac{1}{2} \tr{
            \left( \Kb_{\XbC,\XbC} + \Sigma_{\betabC} \right)^{-1} \Kb_{\XbC,\XbC}}  \\
        & \qquad + \frac{1}{2} \log\left|\Sigma_{\betabC}\right| - \frac{1}{2} \log\left|\Kb_{\XbC,\XbC} + \Sigma_{\betabC}\right| \\
        & \qquad -\frac{1}{2} \ybC^\top (\Kb_{\XbC,\XbC} + \Sigma_{\betabC})^{-1} \Kb_{\XbC,\XbC} (\Kb_{\XbC,\XbC} + \Sigma_{\betabC})^{-1} \ybC \label{eq:data_quadratic_short}
\end{align}

Where for the simplification from Equation~\eqref{eq:data_quadratic_long} to Equation~\eqref{eq:data_quadratic_short} we replaced the coreset-based $\gp$ latent variable's expected value
\begin{align}
	\mb_{\fbC|\ybC} &= \Kb_{\XbC,\XbC}\Kb_{\XbC,\XbC}^{-1} \mb_{\fbC|\ybC} \\
	&= \Kb_{\XbC,\XbC}\Kb_{\XbC,\XbC}^{-1} \Kb_{\fbC|\ybC} \Sigma_{\betabC}^{-1} \ybC \\
	&= \Kb_{\XbC,\XbC}\Kb_{\XbC,\XbC}^{-1} \left( \Kb_{\XbC,\XbC}^{-1} + \Sigma_{\betabC}^{-1} \right)^{-1} \Sigma_{\betabC}^{-1} \ybC \\
		& \qquad \text{ by using equivalence in Equation~\eqref{eq:equiv_1}} \nonumber \\
	&= \Kb_{\XbC,\XbC}\left( \Kb_{\XbC,\XbC} + \Sigma_{\betabC} \right)^{-1} \ybC  \; ,
\end{align} 
and rewrite the quadratic term as
\begin{align}
	& (\ybC-\mb_{\fbC|\ybC})^\top \Sigma_{\betabC}^{-1}(\ybC-\mb_{\fbC|\ybC}) 
            - \ybC^\top (\Kb_{\XbC,\XbC} + \Sigma_{\betabC})^{-1}\ybC = \\
        % Newline
        & \quad = (\ybC^\top-\ybC^\top \left( \Kb_{\XbC,\XbC} + \Sigma_{\betabC} \right)^{-1} \Kb_{\XbC,\XbC}) \Sigma_{\betabC}^{-1}(\ybC-\Kb_{\XbC,\XbC}\left( \Kb_{\XbC,\XbC} + \Sigma_{\betabC} \right)^{-1} \ybC) \nonumber \\
            & \qquad - \ybC^\top (\Kb_{\XbC,\XbC} + \Sigma_{\betabC})^{-1}\ybC \\
        % Newline
        & \quad = \ybC^\top (\Ib_M- \left( \Kb_{\XbC,\XbC} + \Sigma_{\betabC} \right)^{-1} \Kb_{\XbC,\XbC}) \Sigma_{\betabC}^{-1}(\Ib_M-\Kb_{\XbC,\XbC}\left( \Kb_{\XbC,\XbC} + \Sigma_{\betabC} \right)^{-1}) \ybC \nonumber \\
            & \qquad - \ybC^\top (\Kb_{\XbC,\XbC} + \Sigma_{\betabC})^{-1} \ybC \\
        % Newline
        & \quad = \ybC^\top \left[
            (\Ib_M- \left( \Kb_{\XbC,\XbC} + \Sigma_{\betabC} \right)^{-1} \Kb_{\XbC,\XbC}) \Sigma_{\betabC}^{-1}(\Ib_M-\Kb_{\XbC,\XbC}\left( \Kb_{\XbC,\XbC} + \Sigma_{\betabC} \right)^{-1}) 
                - (\Kb_{\XbC,\XbC} + \Sigma_{\betabC})^{-1} 
            \right]\ybC \\
        % Newline
        & \quad = \ybC^\top \left[
            \Sigma_{\betabC}^{-1} 
            - \left( \Kb_{\XbC,\XbC} + \Sigma_{\betabC} \right)^{-1} \Kb_{\XbC,\XbC} \Sigma_{\betabC}^{-1} 
            - \Sigma_{\betabC}^{-1} \Kb_{\XbC,\XbC}\left( \Kb_{\XbC,\XbC} + \Sigma_{\betabC} \right)^{-1})  \right. \nonumber \\
            & \qquad \qquad \left.+ \left( \Kb_{\XbC,\XbC} + \Sigma_{\betabC} \right)^{-1} \Kb_{\XbC,\XbC} \Sigma_{\betabC}^{-1} \Kb_{\XbC,\XbC}\left( \Kb_{\XbC,\XbC} + \Sigma_{\betabC} \right)^{-1})  
            - (\Kb_{\XbC,\XbC} + \Sigma_{\betabC})^{-1} 
            \right]\ybC \\
        % Newline
        & \quad = \ybC^\top \left[
            \Sigma_{\betabC}^{-1} (\Kb_{\XbC,\XbC} + \Sigma_{\betabC})
            - \left( \Kb_{\XbC,\XbC} + \Sigma_{\betabC} \right)^{-1} \Kb_{\XbC,\XbC} \Sigma_{\betabC}^{-1} (\Kb_{\XbC,\XbC} + \Sigma_{\betabC})
            - \Sigma_{\betabC}^{-1} \Kb_{\XbC,\XbC}  \right. \nonumber \\
            & \qquad \qquad \left.+ \left( \Kb_{\XbC,\XbC} + \Sigma_{\betabC} \right)^{-1} \Kb_{\XbC,\XbC} \Sigma_{\betabC}^{-1} \Kb_{\XbC,\XbC} 
            - \Ib
            \right] (\Kb_{\XbC,\XbC} + \Sigma_{\betabC})^{-1} \ybC \\
        % Newline
        & \quad = \ybC^\top (\Kb_{\XbC,\XbC} + \Sigma_{\betabC})^{-1} \left[
            (\Kb_{\XbC,\XbC} + \Sigma_{\betabC}) \Sigma_{\betabC}^{-1} (\Kb_{\XbC,\XbC} + \Sigma_{\betabC}) \right. \nonumber \\
            & \hspace{30ex}\left. - \Kb_{\XbC,\XbC} \Sigma_{\betabC}^{-1} (\Kb_{\XbC,\XbC} + \Sigma_{\betabC})\right. \nonumber \\
            & \hspace{30ex}\left. - (\Kb_{\XbC,\XbC} + \Sigma_{\betabC}) \Sigma_{\betabC}^{-1} \Kb_{\XbC,\XbC}  \right. \nonumber \\
            & \hspace{30ex} \left.+ \Kb_{\XbC,\XbC} \Sigma_{\betabC}^{-1} \Kb_{\XbC,\XbC} 
            - (\Kb_{\XbC,\XbC} + \Sigma_{\betabC})
            \right] (\Kb_{\XbC,\XbC} + \Sigma_{\betabC})^{-1} \ybC \\
        % Newline
        & \quad = \ybC^\top (\Kb_{\XbC,\XbC} + \Sigma_{\betabC})^{-1} \left[
            \Kb_{\XbC,\XbC}\Sigma_{\betabC}^{-1} \Kb_{\XbC,\XbC} + \Kb_{\XbC,\XbC} + \Kb_{\XbC,\XbC} + \Sigma_{\betabC}^{-1}  \right. \nonumber \\
            & \hspace{30ex}\left. - \Kb_{\XbC,\XbC} \Sigma_{\betabC}^{-1} \Kb_{\XbC,\XbC} - \Kb_{\XbC,\XbC} \right. \nonumber \\
            & \hspace{30ex}\left. - \Kb_{\XbC,\XbC} \Sigma_{\betabC}^{-1} \Kb_{\XbC,\XbC} - \Kb_{\XbC,\XbC}  \right. \nonumber \\
            & \hspace{30ex} \left.+ \Kb_{\XbC,\XbC} \Sigma_{\betabC}^{-1} \Kb_{\XbC,\XbC} 
            - \Kb_{\XbC,\XbC} - \Sigma_{\betabC})
            \right] (\Kb_{\XbC,\XbC} + \Sigma_{\betabC})^{-1} \ybC \\
        % Newline
        & \quad = \ybC^\top (\Kb_{\XbC,\XbC} + \Sigma_{\betabC})^{-1} \left[ - \Kb_{\XbC,\XbC} \right] (\Kb_{\XbC,\XbC} + \Sigma_{\betabC})^{-1} \ybC \\
        % Newline
        & \quad = - \ybC^\top (\Kb_{\XbC,\XbC} + \Sigma_{\betabC})^{-1} \Kb_{\XbC,\XbC} (\Kb_{\XbC,\XbC} + \Sigma_{\betabC})^{-1} \ybC 
\end{align} 
